# Supplementary material for: Reproducibility of density functional approximations: how new functionals should be reported
Source: arXiv:2307.07474 ancillary file (2023-08-23)
Supplement: Supplementary file 1 [file SI.pdf]

# Supporting information for "Reproducibility of density functional approximations: how new functionals should be reported"

Susi Lehtola[1, 2] and Miguel A. L. Marques[3]

[1)] *Molecular Sciences Software Institute, Blacksburg, Virginia 24061, United States*

[2)] *Department of Chemistry, University of Helsinki, P.O. Box 55, FI-00014 University of Helsinki, Finland*

[3)] *Research Center Future Energy Materials and Systems of the University Alliance Ruhr, Faculty of Mechanical Engineering, Ruhr University Bochum, Universit"atsstraße 150, D-44801 Bochum, Germany*

The convergence plots for the PW92 functional and the HF and SCF electron densities are given in in fig. 1 for the def2-SVP basis set, in fig. 2 for the def2-TZVP basis set, and in fig. 3 for the AHGBS-9 basis set.

The convergence plots for the PBE functional and the HF and SCF electron densities are given in in fig. 4 for the def2-SVP basis set, in fig. 5 for the def2-TZVP basis set, and in fig. 6 for the AHGBS-9 basis set.

The convergence plots for the TPSS functional and the HF and SCF electron densities are given in in fig. 7 for the def2-SVP basis set, in fig. 8 for the def2-TZVP basis set, and in fig. 9 for the AHGBS-9 basis set.

The convergence plots for the MS0 functional and the HF and SCF electron densities are given in in fig. 10 for the def2-SVP basis set, in fig. 11 for the def2-TZVP basis set, and in fig. 12 for the AHGBS-9 basis set.

The convergence plots for the MVS functional and the HF and SCF electron densities are given in in fig. 13 for the def2-SVP basis set, in fig. 14 for the def2-TZVP basis set, and in fig. 15 for the AHGBS-9 basis set.

The convergence plots for the SCAN functional and the HF and SCF electron densities are given in in fig. 16 for the def2-SVP basis set, in fig. 17 for the def2-TZVP basis set, and in fig. 18 for the AHGBS-9 basis set.

The convergence plots for the r$^2$SCAN functional and the HF and SCF electron densities are given in in fig. 19 for the def2-SVP basis set, in fig. 20 for the def2-TZVP basis set, and in fig. 21 for the AHGBS-9 basis set.

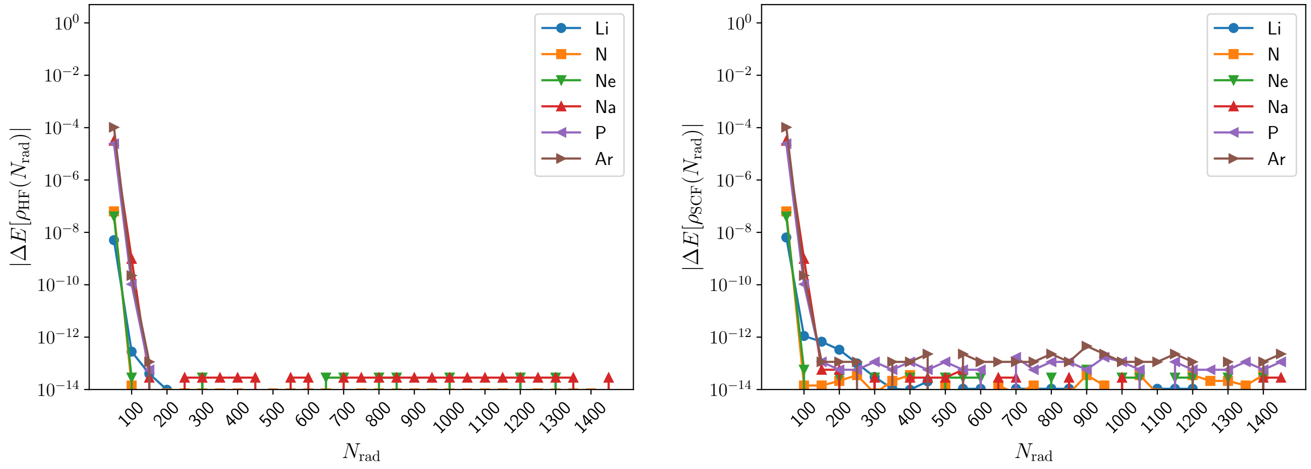


Figure 1. Convergence of the total energies of the Li, N, Ne, Na, P, and Ar atoms with respect to the radial quadrature, employing the PW92 functional, the def2-SVP basis set, and either the HF (left) or the SCF (right) electron density.

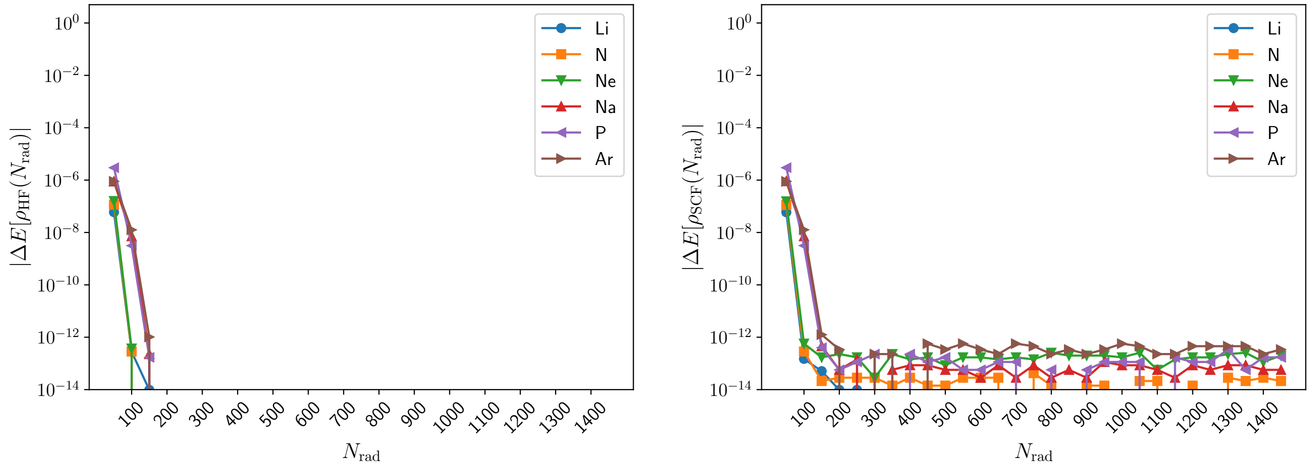


Figure 2. Convergence of the total energies of the Li, N, Ne, Na, P, and Ar atoms with respect to the radial quadrature, employing the PW92 functional, the def2-TZVP basis set, and either the HF (left) or the SCF (right) electron density.

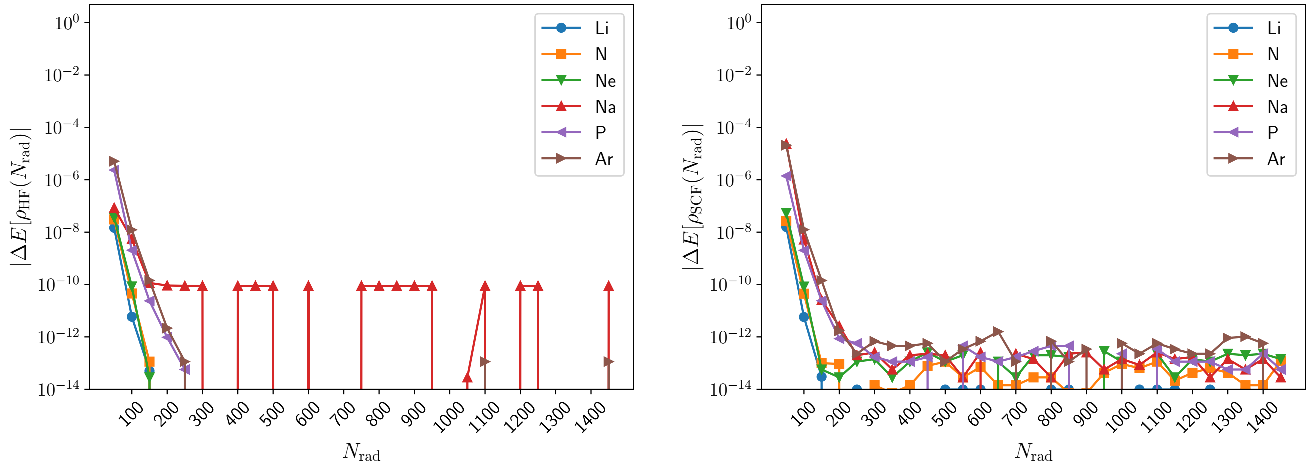


Figure 3. Convergence of the total energies of the Li, N, Ne, Na, P, and Ar atoms with respect to the radial quadrature, employing the PW92 functional, the AHGBS-9 basis set, and either the HF (left) or the SCF (right) electron density.

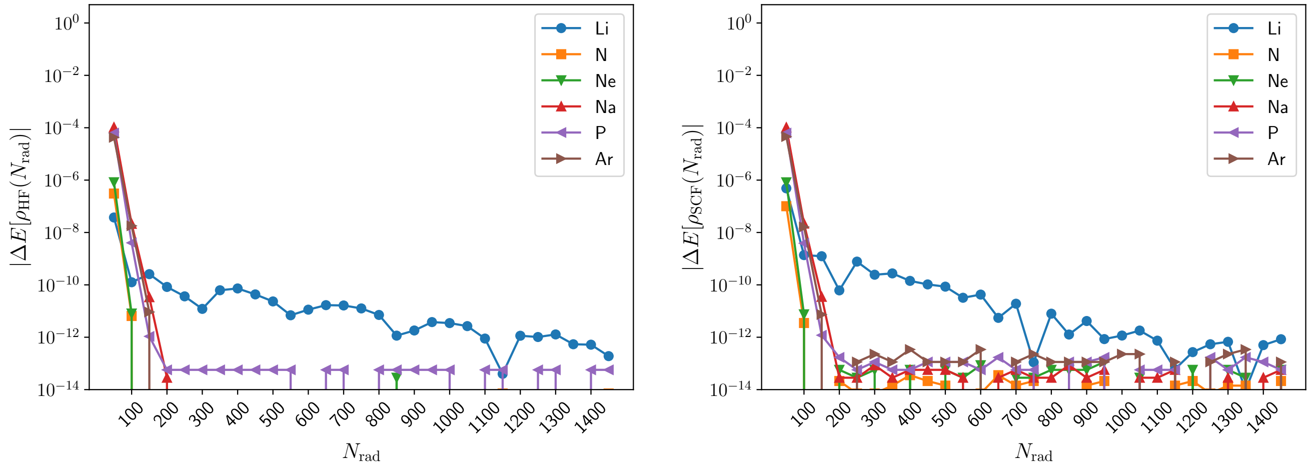


Figure 4. Convergence of the total energies of the Li, N, Ne, Na, P, and Ar atoms with respect to the radial quadrature, employing the PBE functional, the def2-SVP basis set, and either the HF (left) or the SCF (right) electron density.

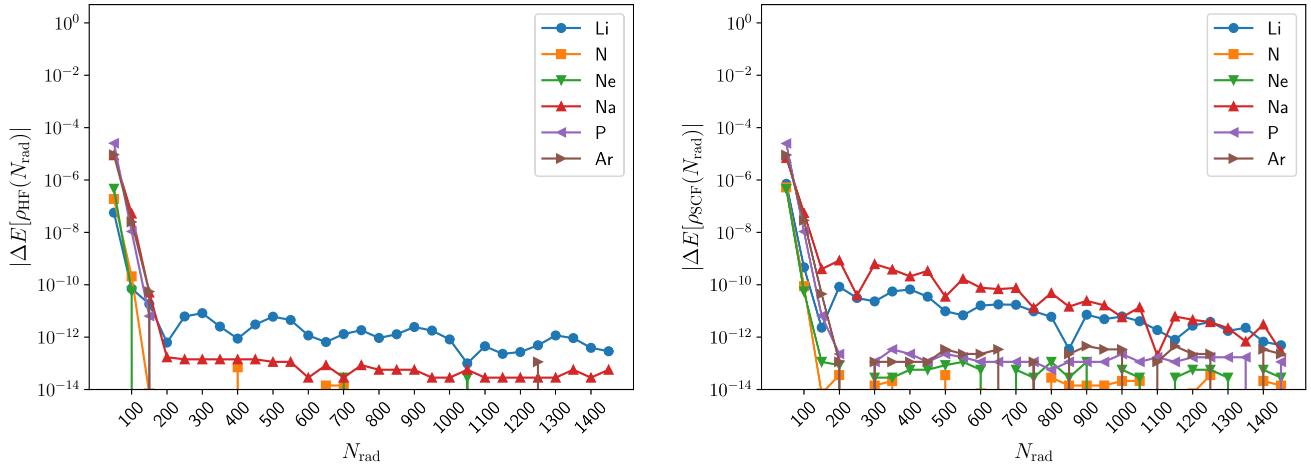


Figure 5. Convergence of the total energies of the Li, N, Ne, Na, P, and Ar atoms with respect to the radial quadrature, employing the PBE functional, the def2-TZVP basis set, and either the HF (left) or the SCF (right) electron density.

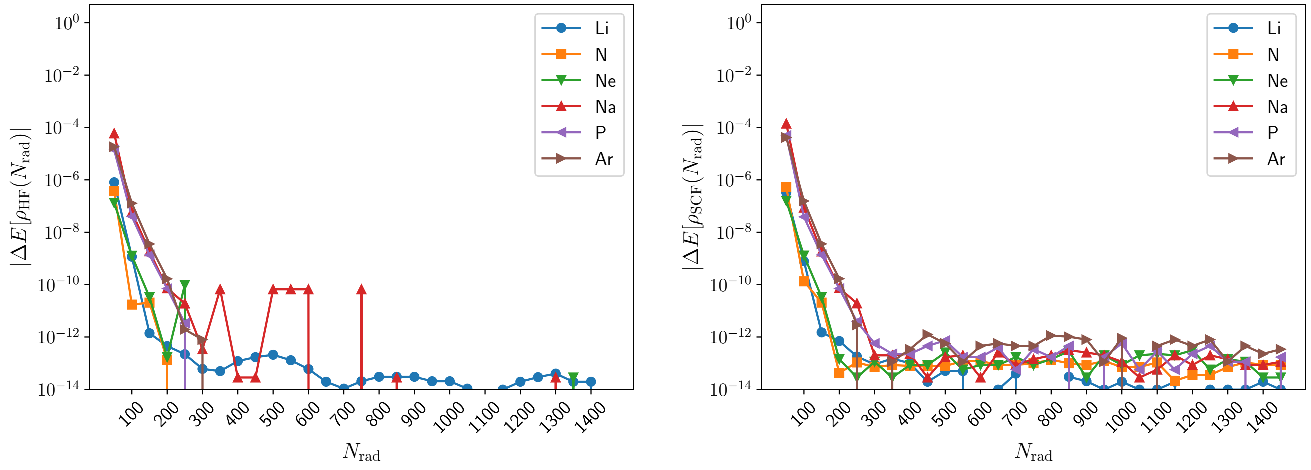


Figure 6. Convergence of the total energies of the Li, N, Ne, Na, P, and Ar atoms with respect to the radial quadrature, employing the PBE functional, the AHGBS-9 basis set, and either the HF (left) or the SCF (right) electron density.

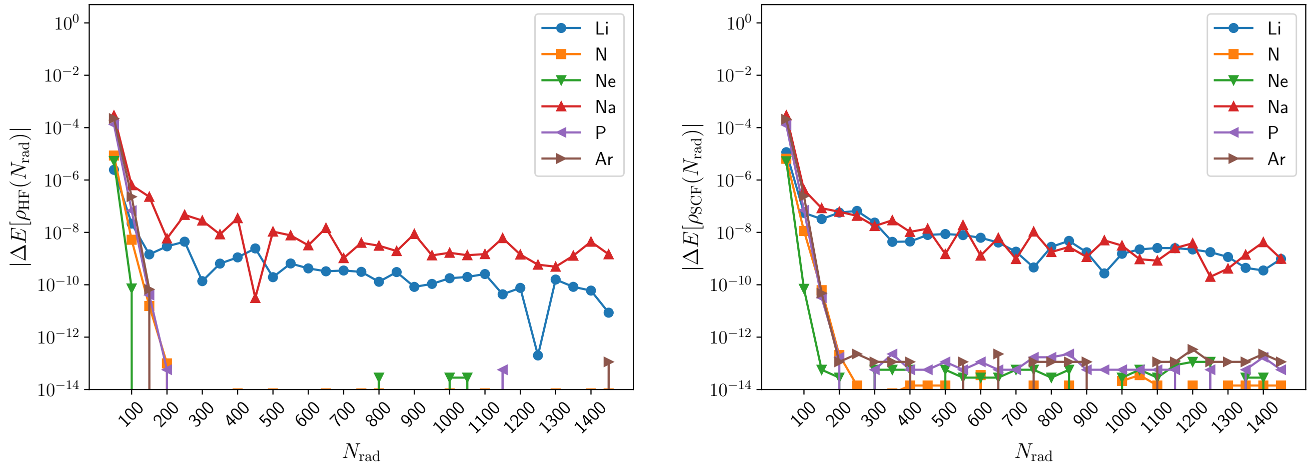


Figure 7. Convergence of the total energies of the Li, N, Ne, Na, P, and Ar atoms with respect to the radial quadrature, employing the TPSS functional, the def2-SVP basis set, and either the HF (left) or the SCF (right) electron density.

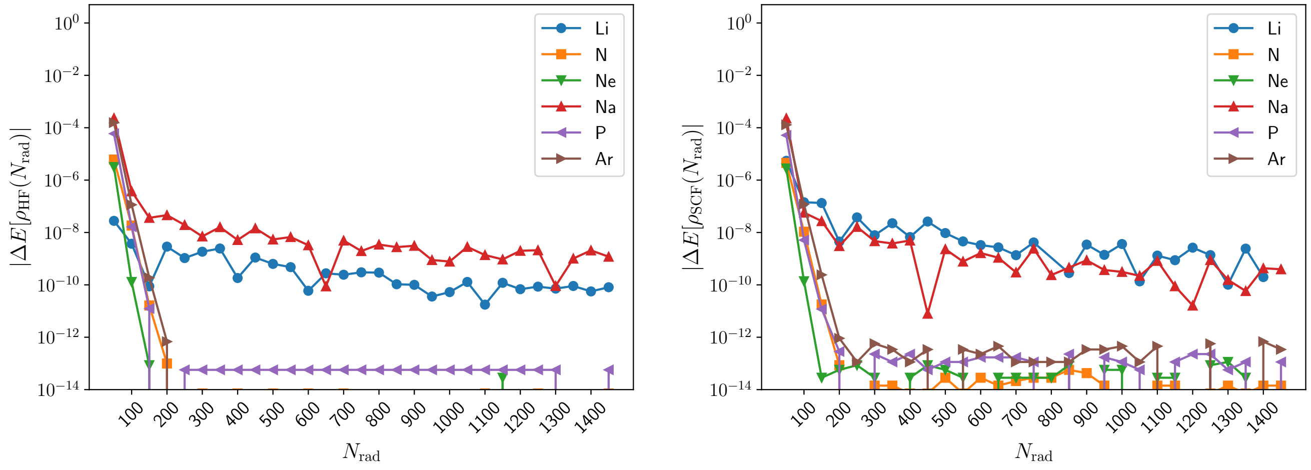


Figure 8. Convergence of the total energies of the Li, N, Ne, Na, P, and Ar atoms with respect to the radial quadrature, employing the TPSS functional, the def2-TZVP basis set, and either the HF (left) or the SCF (right) electron density.

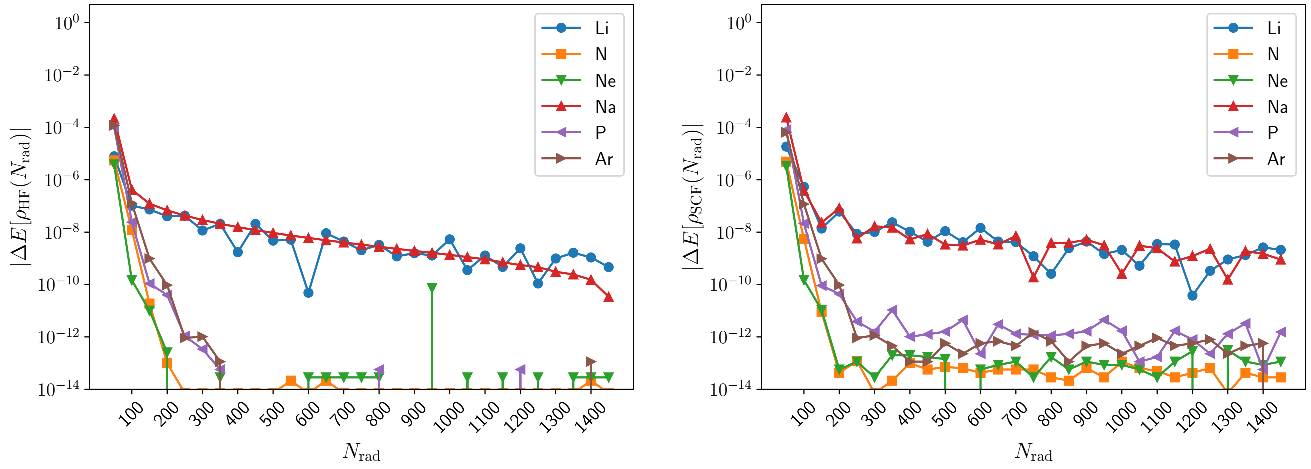


Figure 9. Convergence of the total energies of the Li, N, Ne, Na, P, and Ar atoms with respect to the radial quadrature, employing the TPSS functional, the AHGBS-9 basis set, and either the HF (left) or the SCF (right) electron density.

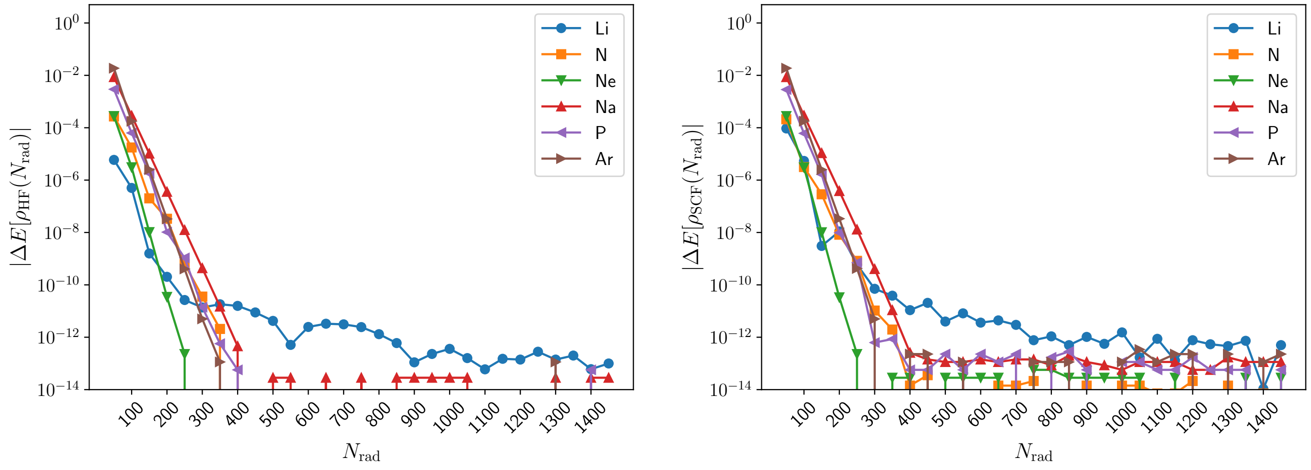


Figure 10. Convergence of the total energies of the Li, N, Ne, Na, P, and Ar atoms with respect to the radial quadrature, employing the MS0 functional, the def2-SVP basis set, and either the HF (left) or the SCF (right) electron density.

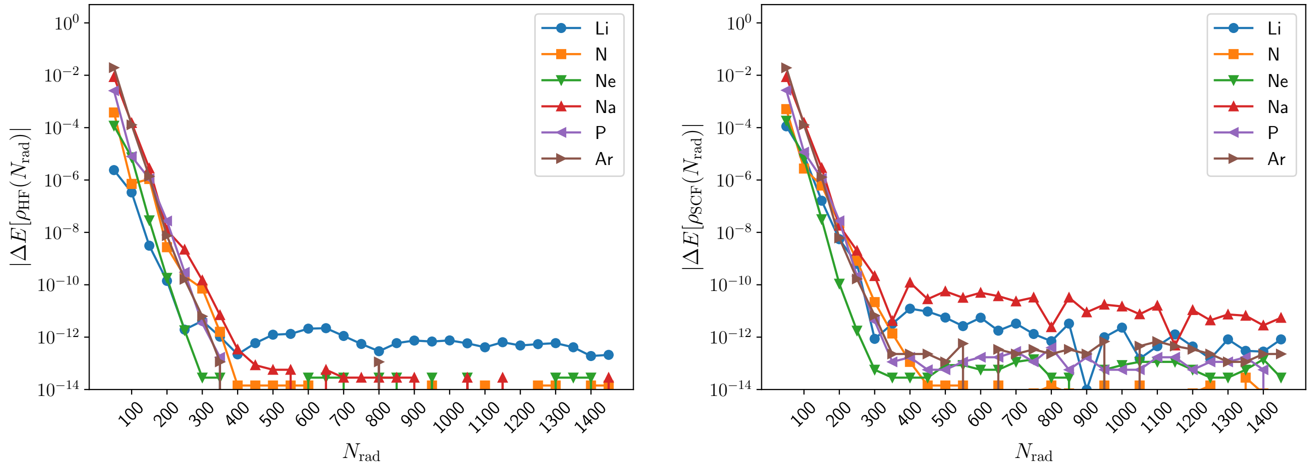


Figure 11. Convergence of the total energies of the Li, N, Ne, Na, P, and Ar atoms with respect to the radial quadrature, employing the MS0 functional, the def2-TZVP basis set, and either the HF (left) or the SCF (right) electron density.

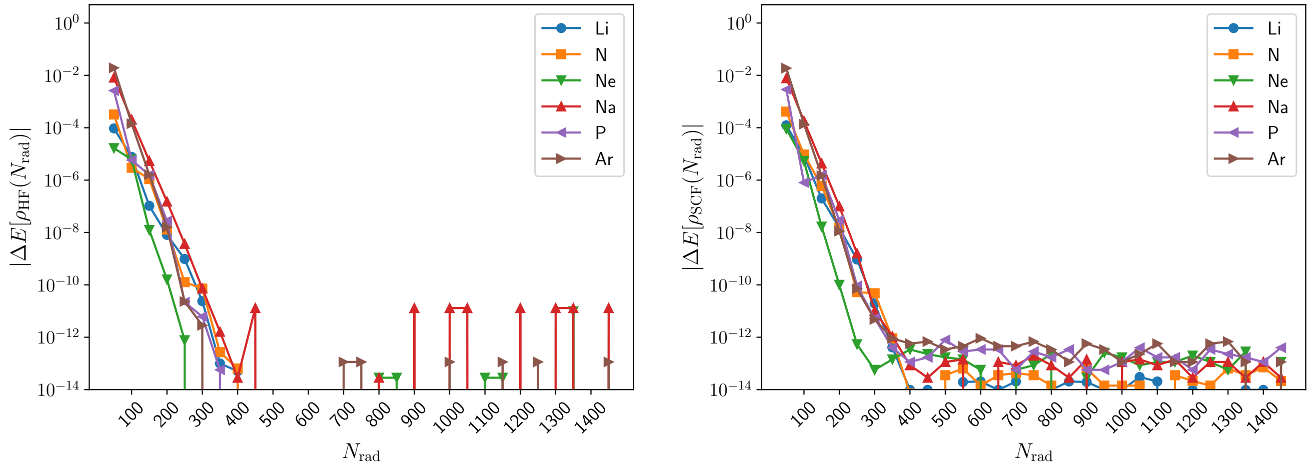


Figure 12. Convergence of the total energies of the Li, N, Ne, Na, P, and Ar atoms with respect to the radial quadrature, employing the MS0 functional, the AHGBS-9 basis set, and either the HF (left) or the SCF (right) electron density.

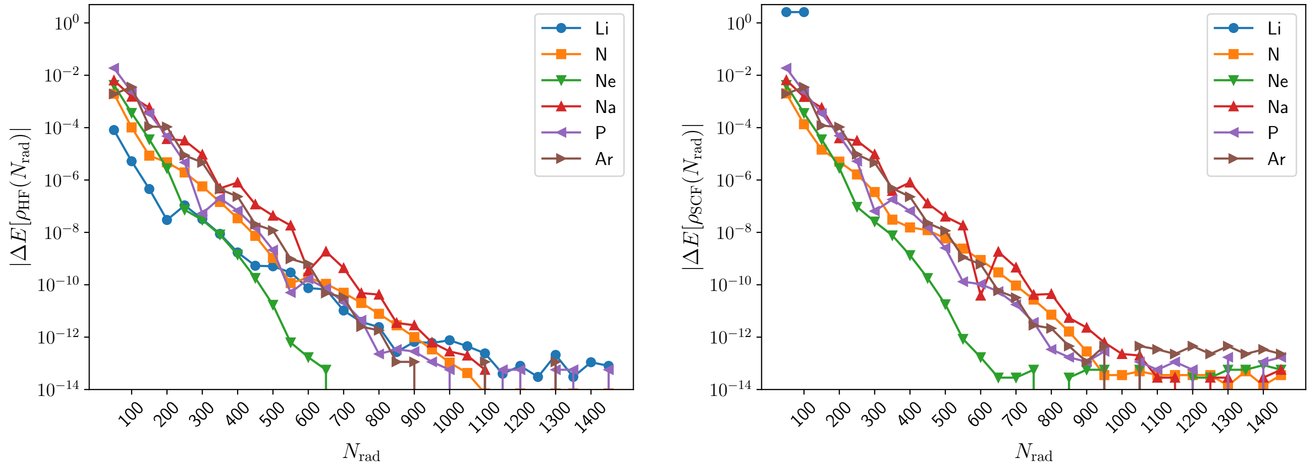


Figure 13. Convergence of the total energies of the Li, N, Ne, Na, P, and Ar atoms with respect to the radial quadrature, employing the MVS functional, the def2-SVP basis set, and either the HF (left) or the SCF (right) electron density.

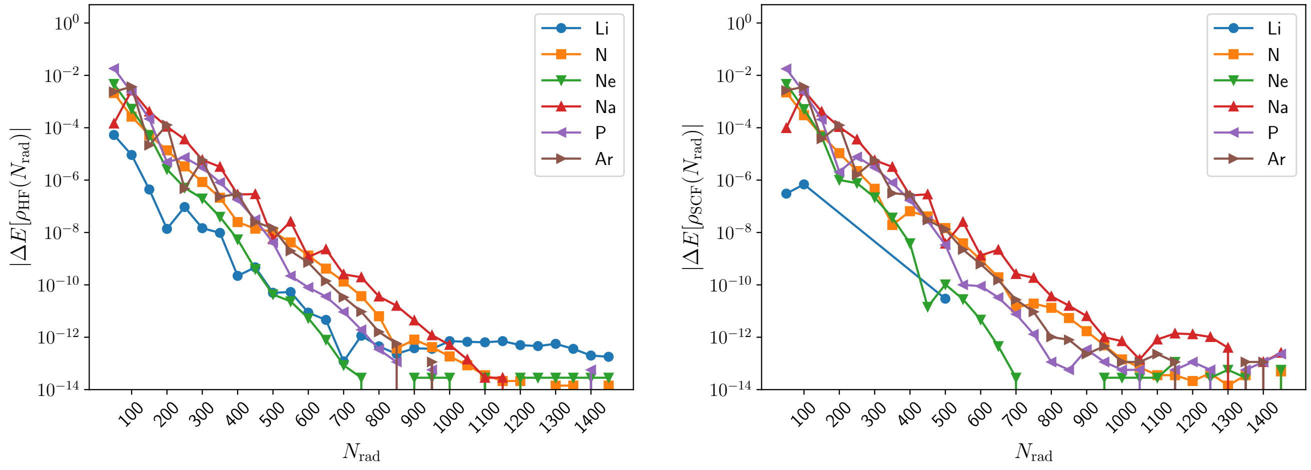


Figure 14. Convergence of the total energies of the Li, N, Ne, Na, P, and Ar atoms with respect to the radial quadrature, employing the MVS functional, the def2-TZVP basis set, and either the HF (left) or the SCF (right) electron density.

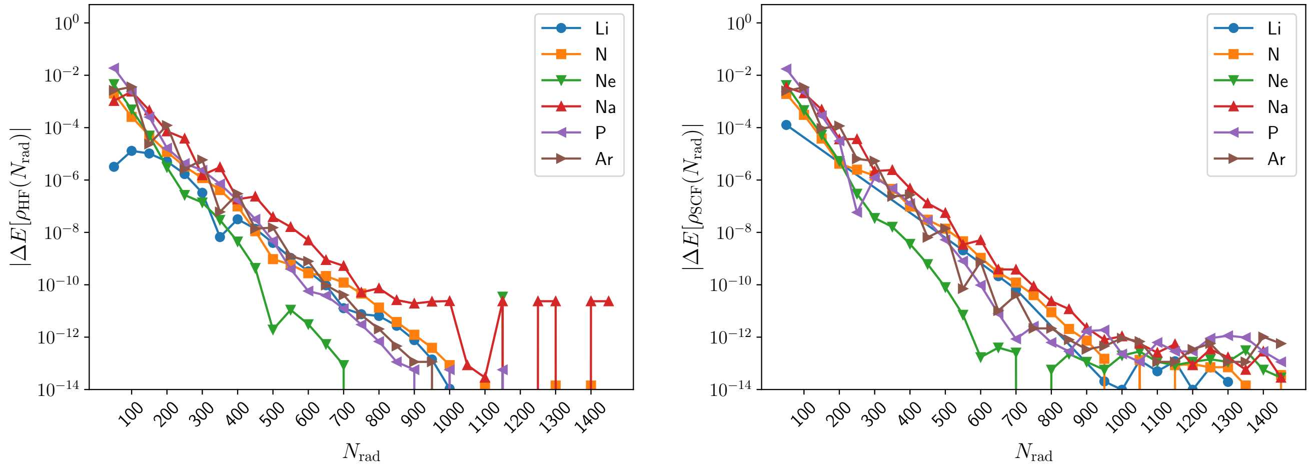


Figure 15. Convergence of the total energies of the Li, N, Ne, Na, P, and Ar atoms with respect to the radial quadrature, employing the MVS functional, the AHGBS-9 basis set, and either the HF (left) or the SCF (right) electron density.

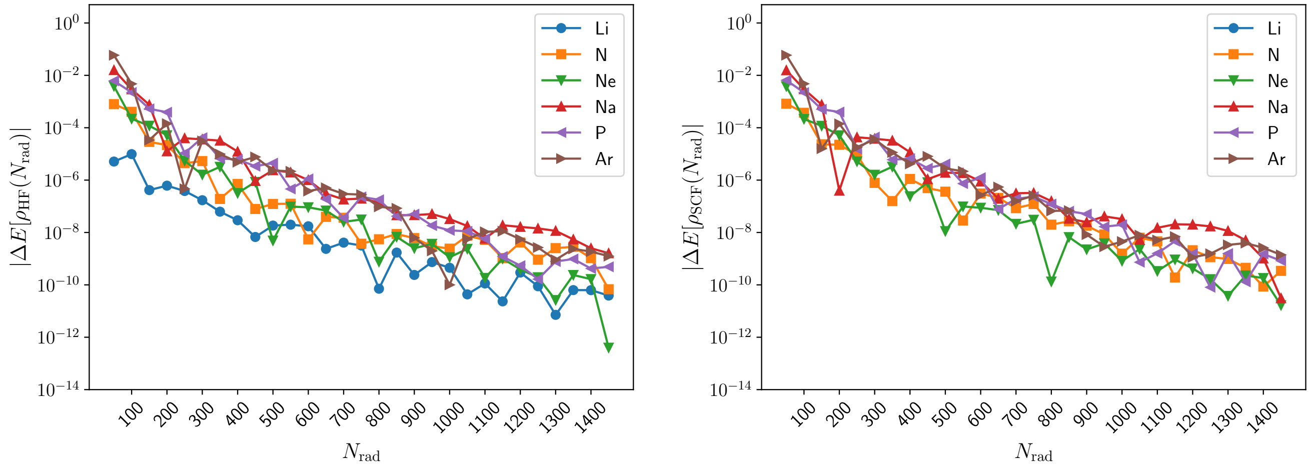


Figure 16. Convergence of the total energies of the Li, N, Ne, Na, P, and Ar atoms with respect to the radial quadrature, employing the SCAN functional, the def2-SVP basis set, and either the HF (left) or the SCF (right) electron density.

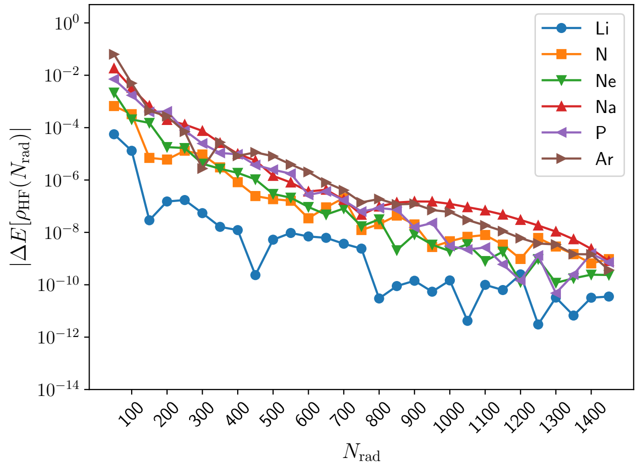


Figure 17. Convergence of the total energies of the Li, N, Ne, Na, P, and Ar atoms with respect to the radial quadrature, employing the SCAN functional, the def2-TZVP basis set, and either the HF (left) or the SCF (right) electron density.

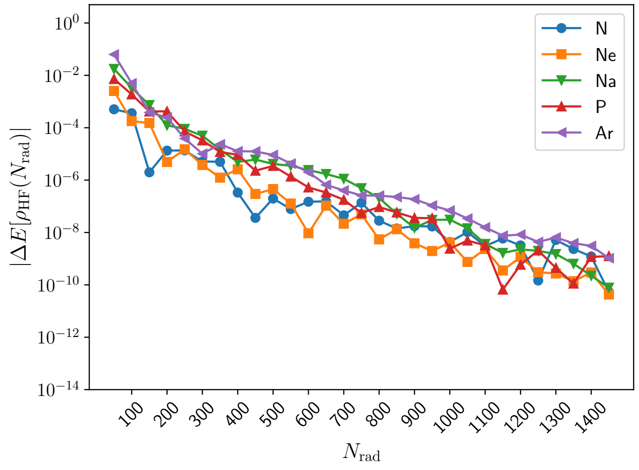


Figure 18. Convergence of the total energies of the Li, N, Ne, Na, P, and Ar atoms with respect to the radial quadrature, employing the SCAN functional, the AHGBS-9 basis set, and either the HF (left) or the SCF (right) electron density.

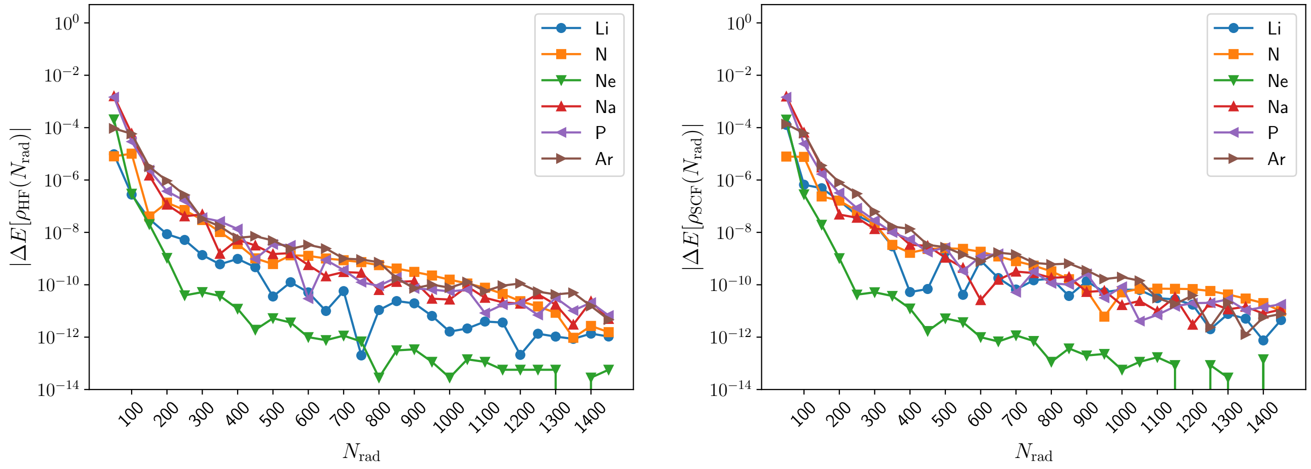


Figure 19. Convergence of the total energies of the Li, N, Ne, Na, P, and Ar atoms with respect to the radial quadrature, employing the r$^2$SCAN functional, the def2-SVP basis set, and either the HF (left) or the SCF (right) electron density.

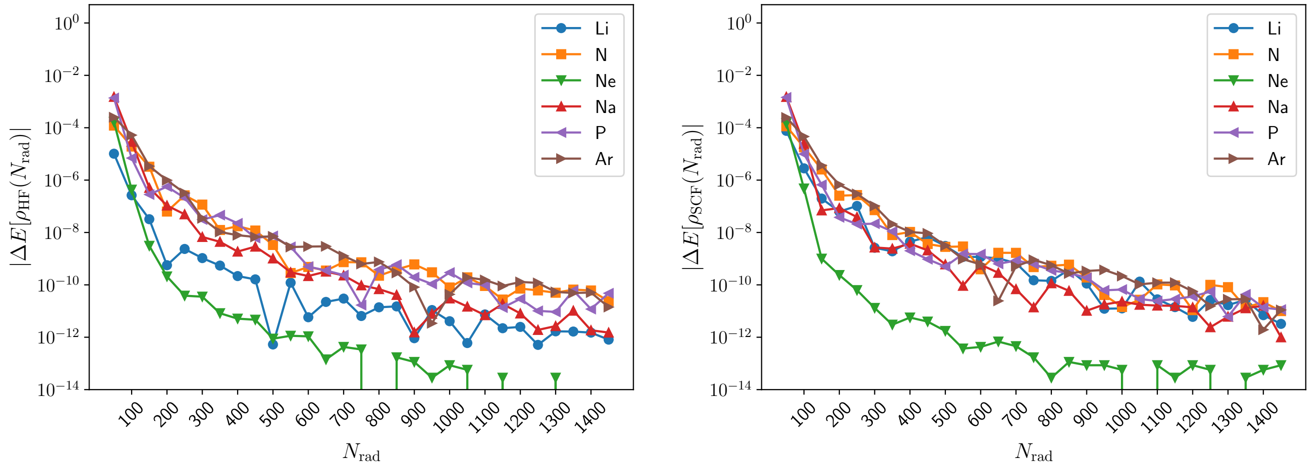


Figure 20. Convergence of the total energies of the Li, N, Ne, Na, P, and Ar atoms with respect to the radial quadrature, employing the r$^2$SCAN functional, the def2-TZVP basis set, and either the HF (left) or the SCF (right) electron density.

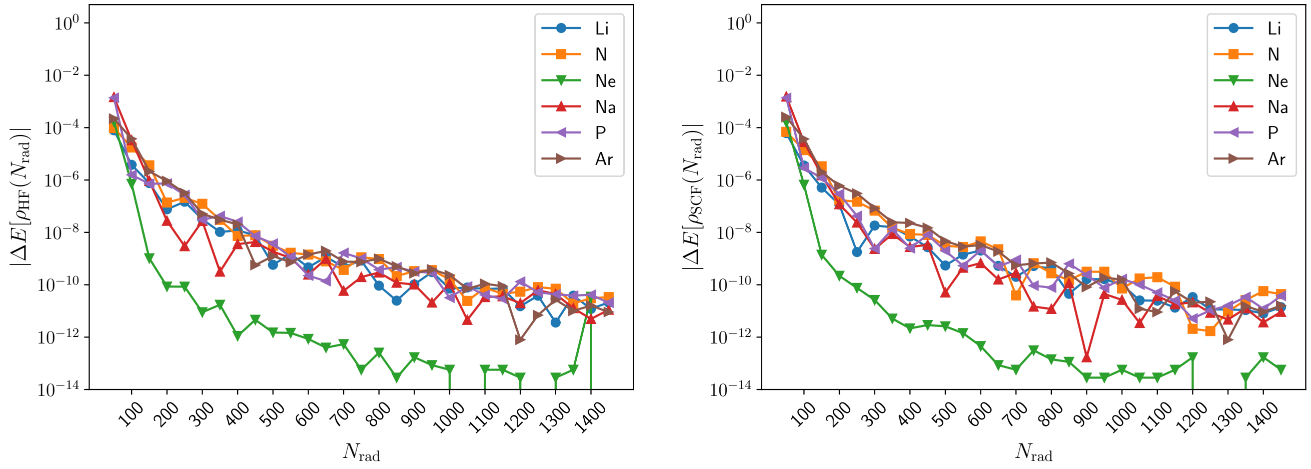


Figure 21. Convergence of the total energies of the Li, N, Ne, Na, P, and Ar atoms with respect to the radial quadrature, employing the r$^2$SCAN functional, the AHGBS-9 basis set, and either the HF (left) or the SCF (right) electron density.
